# Supplementary material for: 3D Projection Sideband Cooling
Source: arXiv:1202.6631 source file (2012-02-29)
Supplement: Supplementary file 1 [file Supplement.pdf]

# Supplemental Material for "3D Projection Sideband Cooling"

Xiao Li, Theodore A. Corcovilos, Yang Wang, and David S. Weiss
Physics Department, The Pennsylvania State University, 104 Davey Lab, University Park, PA, 16803 USA

## Experimental geometry

Our experiment was previously described in Ref. [1]. Of particular relevance to this Letter is the direction of the magnetic bias field (red arrow in Fig. S1). In order for polarization rotation of the lattice beams (blue arrows in Fig. S1) to relatively translate the $F = 3$, $m_F = -3$ and $F = 4$, $m_F = -4$ states, the quantization axis must have a nonzero projection onto the propagation direction of the lattice beams. For our lattice beam geometry, the projection of the magnetic field onto all 3 lattice axes is maximized by placing it in the *x*-*y* plane at 45° to the *x* axis. The optical pumping beam is aligned parallel to the field to ensure that only $\sigma_-$ transitions are driven during optical pumping. Imaging (Fig. 1 of the main text) is along the *z* axis.

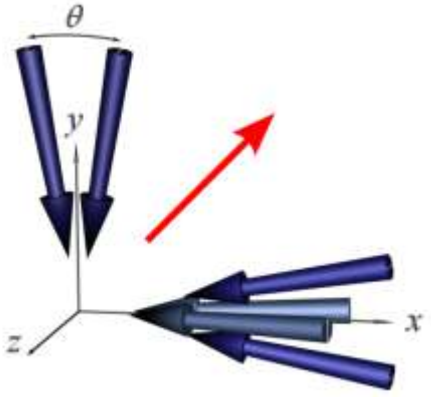


Figure S 1 – Schematic of the experimental geometry. The blue arrows indicate the directions of the optical lattice beams. The pair of beams for each axis is separated by an angle θ = 10°. The nominal polarization of each pair of lattice beams is normal to the plane of propagation of the pair. The red arrow shows the direction of the bias magnetic field, which lies in the *x*-*y* plane at 45° to the *x* axis.

## Projection sideband cooling matrix elements

### State-dependent displacement

We displace the lattice potentials of the hyperfine sublevels $F = 4$, $m_F = -4$ and $F = 3$, $m_F = -3$ by rotating the linear polarization of one of the laser beams which generate the lattice along a given axis[2]. This creates an imbalance in the intensities of the $\sigma_+$ and $\sigma_-$ polarizations of the lattice light. Because the Clebsch-Gordan coefficients to the nearest excited state ($6P_{3/2}$) are different for the two sublevels, the relative potentials of the two states are shifted. The calculated displacement of the potentials as a function of the polarization rotation is shown in Fig. S2. In our experiment we use a rotation of 5.4°, which corresponds to a relative linear displacement of 35 nm.

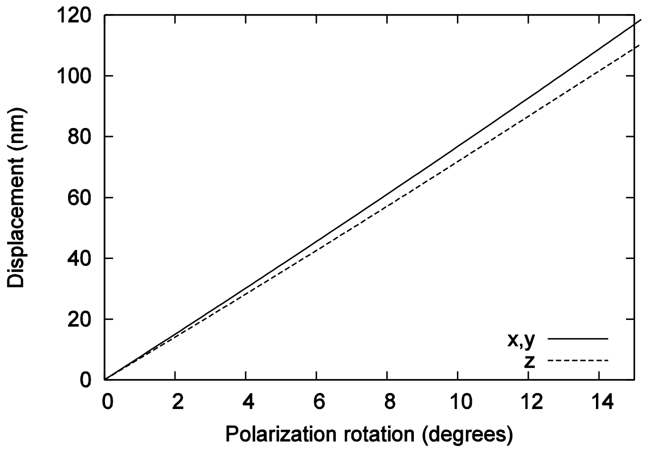


Figure S 2 – Relative position displacement of the $F$ = 4, $m_F$ = -4 and $F$ = 3, $m_F$ = -3 hyperfine sublevels as a function of the lattice polarization rotation angle for the three lattice axes.

## Matrix elements

Given the relative displacement $\Delta x$ of the potentials for the F = 4 and F = 3 states, the spatial overlap integrals

$$A_{n_i,m_i} = \int_{-\infty}^{\infty} \psi^*_{m_i}(x + \Delta x)\psi_{n_i}(x)\, dx,$$

determine the coupling between vibrational states, where $\psi_j$(x) is the $j$-th 1D harmonic oscillator eigenfunction. The values of $A_{n_i,n_i+\Delta n_i}$ for the displacement used in our experiment are shown in Fig. S3. Efficient microwave transitions require $|A_{n_i,n_i+\Delta n_i}| > 0.1$ (discussed below). Note that the nodes for $\Delta n_i$ = 1 and $\Delta n_i$ = 2 occur at different values of $n_i$. There is therefore at least one efficient microwave transition from every vibrational level, and atoms do not get stuck in high-lying $n_i$ levels.

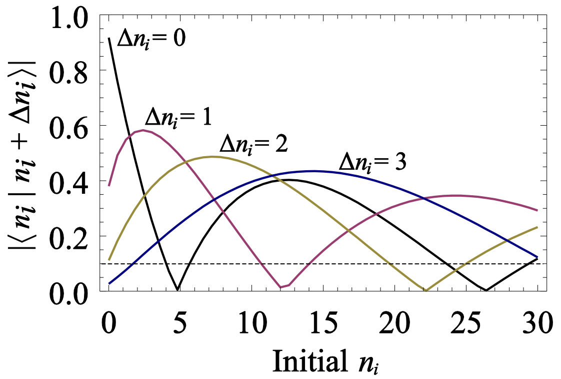


Figure S 3 - Overlap amplitude $|\langle n_i | n_i + \Delta n_i \rangle|$ when the initial and final states have a relative spatial displacement of 0.59 of the harmonic oscillator length. The horizontal dashed line represents the minimum value needed for >98% microwave transfer using adiabatic fast passage with our experimental parameters. Note that at least one of the $\Delta n_i$ = 1 or 2 amplitudes is above the threshold for all values of $n_i$.

## Adiabatic Fast Passage microwave pulses

We implement our microwave transitions using an Adiabatic Fast Passage (AFP) scheme[3]. By shaping the frequency $f$ and power $P$ of the microwave pulse we can calculate >98% transfer efficiency (and measure >96(2)% efficiency) while being insensitive to variations in matrix elements or resonance frequency such as those caused by spatial inhomogeneity or vibrational level dependence. The microwave pulses are generated by a direct digital synthesizer (~100 MHz output, 1 MHz update rate) and then up-converted using a single sideband mixer to the $F$ = 3 to 4 hyperfine resonance (~9.2 GHz), amplified, and then projected onto the atoms with a horn. The frequency and power vary in time according to

$$f(t) = f_0 + \delta f \,\mathrm{sign}\left(\frac{t}{\tau} - \frac{1}{2}\right) \sqrt{1 - \sin^4\left(\frac{\pi t}{\tau}\right)},$$

$$P(t) = P_{max} \,\sin^4\left(\frac{\pi t}{\tau}\right), \qquad \text{(S1)}$$

where $f_0$ is the nominal resonance frequency, $\delta f$ = 4 kHz is half of the chirp range, $\tau$ = 3 ms is the length of the pulse, and $P_{\mathrm{max}}$ is the maximum output power. These time dependences are designed for equal adiabaticity throughout the pulse. The coupling of the microwaves to the atoms is determined empirically by measuring the Rabi frequency of $F$ = 4, $m_F$ = -4 to $F$ = 3, $m_F$ = -3, $\Delta n_i$ = 0 oscillations in the unshifted lattice (2π × 11.1 kHz at maximum output power).

We model the efficiency of the AFP pulses by numerically integrating the Bloch equations for a two-level system with our experimental parameters. The calculation shows that $|A_{n_i,n_i+\Delta n_i}| > 0.1$ is needed for transfer efficiencies of >98%,(Fig. S4(a)). The AFP pulses are insensitive to inhomogeneous frequency broadening up to half the chirp range (Fig. S4(b)). Inhomogeneous broadening will narrow the plateau (e.g. Fig. 3 of the main text) and for broadening much larger than the chirp range, reduce the maximum efficiency. During the cooling sequence the center frequency of the pulse is chosen empirically to maximize the transfer efficiency.

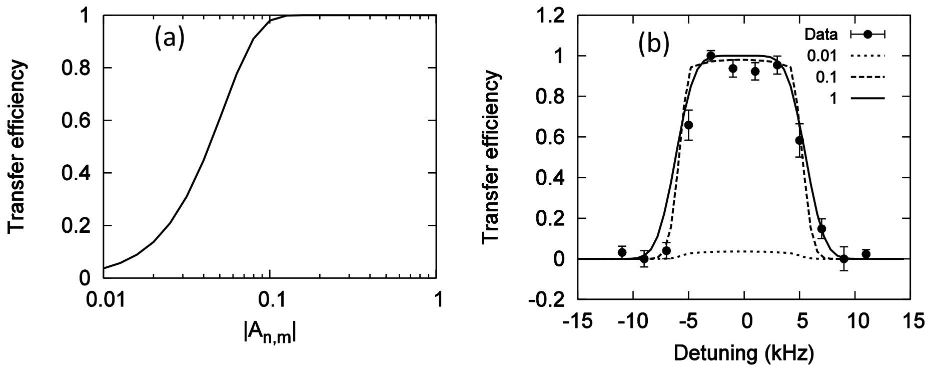


Figure S 4 – (a) Calculated microwave transfer efficiency as a function of spatial overlap. (b) Transfer efficiency as a function of detuning using a chirp range of ±6 kHz. The traces represent the cases of different spatial overlap values: solid line = 1, dashed line = 0.1, and dotted line = 0.01. The filled circles are experimental data with 1σ statistical error bars for the carrier transition ($\Delta n_i$ = 0) without lattice displacement.

## Spontaneous emission from the lattice

It has long been theoretically known that the heating from spontaneous emission in a standing wave does not depend on the atom's location in the standing wave[4]. That result has been recently explicitly derived for quantized motion in an optical lattice[5,6], with the direct implication that the heating rate is the same whether an atom is trapped in a blue detuned lattice at the node or in a red detuned lattice at the antinode. This result does not hold in our geometry, where heating is substantially reduced because the lattice light is blue-detuned. The motional factor in the spontaneous emission rate in a blue-detuned lattice is

$$\left|\langle n_i'|e^{i\boldsymbol{k_s}\cdot\boldsymbol{r}}\sin\left(k_L\boldsymbol{r_i}\sin\left(\tfrac{\theta}{2}\right)\right)|n_i\rangle\right|^2, \qquad \text{(S2)}$$

where $n_i$ and $n_i'$ are initial and final vibrational states. The outer sine term comes from the lattice field, where $\boldsymbol{k_L}$ is the lattice light wavevector, $\theta$ is the relative angle of beams in a lattice pair ($10^o$ in our experiment), and **r** is the position operator with components $r_i$. The exponential factor comes from the electric field of the spontaneously emitted photon with propagation vector $\boldsymbol{k_s}$, and $k_s \approx k_L$. To first order in $\eta$, the Lamb-Dicke parameter, S2 simplifies to

$$\left|\left\langle n_i'\right| k_L r_i \sin\left(\frac{\theta}{2}\right)\left|n_i\right\rangle\right|^2 \qquad \text{(S3)}$$

A standard atomic scattering calculation incorporating S2 shows that the direct heating rate due to spontaneous emission in this lattice is

$$\dot{E} = E_r\frac{\Gamma\Omega^2}{4\delta^2}\sin^2\left(\frac{\theta}{2}\right), \qquad \text{(S4)}$$

where $E_r = (\hbar k_s)^2/2m$ is the photon recoil energy, Γ is the natural linewidth of the nearby optical resonance, Ω is the Rabi frequency for the intensity at the peak of the standing wave, and $\delta$ is the detuning. Heating is suppressed compared to a lattice made from counterpropagating beams by a factor of the ratio of the lattice constants squared.

For a red-detuned lattice, the motional factor in spontaneous emission is

$$\left|\langle n_i'|e^{i\boldsymbol{k_s}\cdot\boldsymbol{r}}\cos\left(k_L r_i\sin\left(\tfrac{\theta}{2}\right)\right)|n_i\rangle\right|^2, \qquad \text{(S5)}$$

which in the Lamb-Dicke limit is approximately

$$|\langle n_i'|\, i\boldsymbol{k_s}\cdot\boldsymbol{r}\,|n_i\rangle|^2. \qquad \text{(S6)}$$

That is, the motional part of spontaneous emission, and thus the heating, is the same as for a lattice made from counterpropagating beams. One can understand the dependence on detuning sign by considering the origin of heating in each case. In a blue-detuned 3D lattice the lattice photons cause most of the heating. These photons heat because of the spatial gradient of their field at the atom, which

is inversely proportional to the lattice constant. While the spontaneously emitted photons are a necessary part of spontaneous emission, in a blue-detuned lattice they only lead to vibrational changes to second order in $\eta^2$. In a red-detuned 3D lattice, the heating roles of the photons are reversed. The spontaneous photon causes vibrational changes to first order, while the stimulated photon does not. The field from the spontaneous photon looks the same regardless of the lattice constant, so heating in a red-detuned lattice is independent of lattice constant.

Total direct heating from the 3D vibrational ground state due to lattice spontaneous emission in our experiment is 1.6 $E_r$ / s (0.22 $\hbar\omega$/ s, where $\hbar\omega$ is the harmonic oscillator energy).

## Optical pumping heating

Optically pumping atoms to the dark state ($F$ = 4, $m_F$ = -4) heats the atoms. Monte Carlo simulations of the optical pumping process shows that an atom in either the $F$=3, $m_F$ = -3 state or the $F$=4, $m_F$ = -3 requires an average of 2.16 spontaneous emissions to return to the dark state. Each spontaneous emission heats by an average $2E_r$, with equal contributions from the absorbed and emitted photons. For our $\eta$, the average heating from optical pumping is 0.24 $\hbar\omega$. Since the stimulated parts of the projection sideband cooling cycle are so efficient, optical pumping heating is the primary limiting factor in the rate at which vibrational energy is removed during the projection sideband cooling cycle.

The heating cost of optical pumping also has the effect of augmenting the heating from spontaneous emission. In a blue-detuned lattice, most spontaneous emission events lead to a change in vibrational level. Depending on how far the light is detuned from the atomic fine structure, spontaneous emission also has a chance to change the atoms' magnetic sublevel. When it does, that atom will be heated by an additional 0.24 $\hbar\omega$. The spontaneous emission rate is

$$\Gamma_{sp} = \frac{\Gamma\Omega^2}{4\delta^2}\eta^2 \sin^2\left(\frac{\theta}{2}\right)\left(1 + 2(n_x + n_y + n_z)\right), \qquad \text{(S7)}$$

so this secondary heating starts to exceed direct spontaneous emission heating when atoms have more than one vibrational quantum of excitation.

When the optical pumping beam is contaminated by the wrong circular polarization, it can drive atoms out of the dark state via the $F'$ = 4, $m_F$ = -3 excited state. In this case, it takes 3.68 spontaneous emissions with average heating of 0.41 $\hbar\omega$ to return to the dark state.

Combining the above results with the calculated lattice scattering rate gives a total lattice heating rate (direct plus optical pumping) of 0.34 $\hbar\omega$ per second from the ground state. It becomes the dominant source of lattice-based heating for larger $n$ (see Fig. S5).

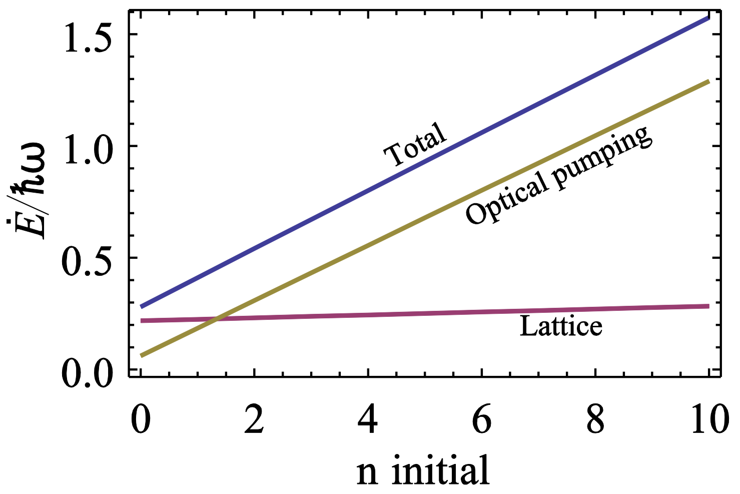


Figure S 5 – Calculated heating rates for heating from the lattice in units of $\hbar\omega$ per second. The red curve indicates the direct heating from spontaneous emission of lattice light. The yellow curve shows heating from optical pumping after a lattice spontaneous emission required to return the atoms to the $F$ = 4, $m_F$ = -4 state. The blue curve is the sum of these effects.

## References

[1] Karl D. Nelson, Xiao Li, and David S. Weiss, Nature Physics **3**, 556-560 (2007).

[2] Ivan H. Deutsch and Poul S. Jessen, Physical Review A **57**, 1972-1986 (1998).

[3] F. Bloch, Physical Review **70**, 460-474 (1946).

[4] J. P. Gordon and A. Ashkin, Physical Review A **21**, 1606-1617 (1980).

[5] H. Pichler, A. Daley, and P. Zoller, Physical Review A **82**, (2010).

[6] Fabrice Gerbier and Yvan Castin, Physical Review A **82**, (2010).
